# Supplementary material for: Nonlinear Hysteretic Torsional Waves
Source: arXiv:1501.02179 source file (2015-01-09)
Supplement: Supplementary file 1 [file SuppMat.pdf]

# Nonlinear Hysteretic Torsional Waves (Supplementary Material)

J. Cabaret, P. Béquin, G. Theocharis,[1] V. Andreev,[2] and V.E. Gusev, V. Tournat[1]

[1]*LUNAM Universités, CNRS, Université du Maine, LAUM UMR-CNRS 6613, Av. O. Messiaen, 72085 Le Mans, France.*

[2]*Acoustics Department, Faculty of Physics, Moscow State University, Moscow, Russia*

(Dated: January 8, 2015)

### Nonlinear moment-angle relationship for torsional contacts

In the first section, the problem of two elastic beads in Hertz contact subjected to oscillating torsional moment is considered. A nonlinear relation between the torsional moment and the angle of rigid rotation which includes the dependence on history of the process (hysteresis and memory) is derived. The calculation is based on the solutions for torsion of elastic spheres in contact that were initiated by Mindlin [1] and extended by Lubkin [2], Deresiewicz [3], Hetényi and McDonald [4].

### Hertzian contact with normal force

Two identical elastic beads are placed in contact under the action of a static normal force $F_0$ (figure 1). The Hertz theory [5] gives the relative displacement of the centers of the two beads

$$\delta = 2\delta_z = 2\left[\frac{F_0^2}{R}\left(\frac{3}{4}\frac{1-\nu^2}{E}\right)^2\right]^{\frac{1}{3}}, \quad (1)$$

where R is the radius of the beads, $E$ and $\nu$ are the Young's modulus and Poisson ratio of the bead's material.

The theory also predicts a plane circular contact surface of radius

$$a = \left[\frac{3}{4}\frac{1-\nu^2}{E}\,R\,F_0\right]^{\frac{1}{3}}. \quad (2)$$

### Additional torsional moment

An additional torsional moment $M_z$ is now applied relative to the axis of normal contact. This moment causes one bead to rotate around the z-axis with a small angle $\beta$ relative to the other bead. The nonlinear relation between this torsional moment and rotation angle was

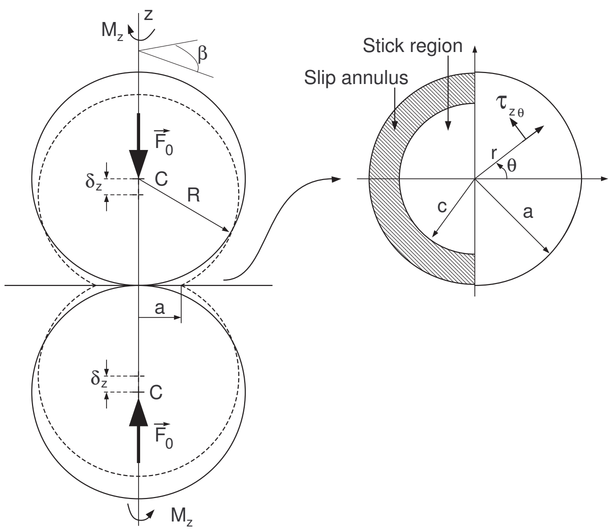


Figure 1. Geometrical configuration of an Hertzian contact with normal force $F_0$ and torsional moment $M_z$. There is coexistence of a slip region ($c \le r \le a$) and stick region ($r \le c$) within the contact surface.

first obtained by Mindlin [1] who found that, in absence of slip at the contact surface, the shear stress $\tau_{z\theta}$ (figure 1) goes to infinity as $r$ approaches $a$, the boundary of the contact. This theory was re-examined by Lubkin [2] to include slip consideration. According to this theory, when a monotonically increasing torsional moment is added to a contact under a static normal force, slip occurs at the contact surface, starting at the circumference of the area of contact and progressing radially inward so that the surface of slip occurence is an annulus of outer radius $a$ and inner radius $c$. After lengthy calculations, Lubkin gives two relationships. The first one is between the angle of rotation $\beta$ and the inner radius $c$,

$$\beta = \frac{\mu F_0}{Ga^2}\frac{3k^2}{4\pi}\mathbf{D}(k^2) \qquad \text{with} \quad k = \sqrt{1-\left(\frac{c}{a}\right)^2} \quad (3)$$

and,

$$\mathbf{D}(k^2) = \frac{\mathbf{K}(k^2) - \mathbf{E}(k^2)}{k^2}, \quad (4)$$

where $\mu$ is the dynamic coefficient of friction, $G = \frac{E}{2(1+\nu)}$. **K** and **E** are, respectively, the complete elliptic integrals of first and second kinds [6].

The second one is the relation between the torsional moment $M_z$ and the inner radius $c$ :

$$M_z = \frac{\mu F_0 a}{4\pi}\Bigg\{\frac{3\pi^2}{4} + k'k^2\big[6\mathbf{K} + (4k'^2 - 3)\mathbf{D}\big] - 3k\mathbf{K}\arcsin k' - 3k^2\Bigg[\mathbf{K}\int_0^{\frac{\pi}{2}} \frac{\arcsin(k'\sin\alpha)}{\big[1-(k'sin\alpha)^2\big]^{\frac{3}{2}}}d\alpha - \mathbf{D}\int_0^{\frac{\pi}{2}} \frac{\arcsin(k'\sin\alpha)}{\big[1-(k'sin\alpha)^2\big]^{\frac{1}{2}}}d\alpha\Bigg]\Bigg\}, \quad (5)$$

with $k' = \frac{c}{a}$.

Figure 2 shows the relation between the torsional moment $M_z$ and the angle $\beta$. As the torsional moment is increased, the stick region shrinks until the onset of free sliding when one bead is then free to spin relative to the other. The value of the torsional moment at which slip occurs over the entire contact surface is $M_z = \frac{3\pi}{16}\mu F_0\, a$, which corresponds to an infinite value of $\beta$.

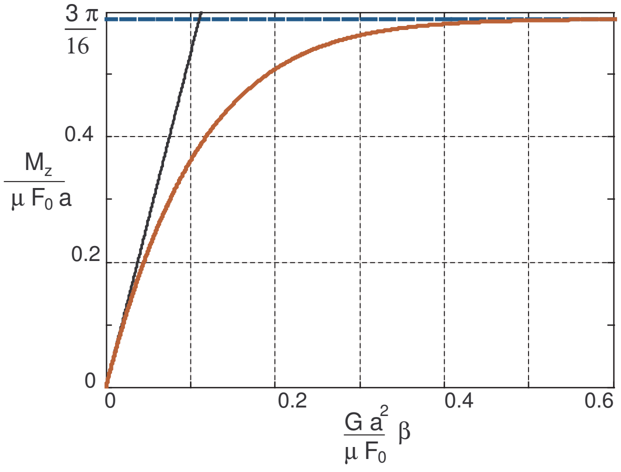


Figure 2. Illustration of the relation between the torsional moment of Eq. (5) and the angle of rotation, Eq. (4). The straight line represents the initial torsional rigidity $K_t = dM_z/d\beta = \frac{16}{3}Ga^3$.

*Approximate relation of Deresiewicz*

In order to establish a wave propagation equation, it is necessary to have an explicit and reversible relation between the torsional moment and the angle of bead rotation. Deresiewicz [3] derived this relation, only applicable for small values of the moment $\frac{M_z}{\mu F_0 a}$, i.e., $c/a \approx 1$,

$$\frac{Ga^2}{\mu F_0}\beta = \frac{1}{8}\left[1-\left(1-\frac{3}{2}\frac{M_z}{\mu F_0 a}\right)^{\frac{1}{2}}\right]\left[3-\left(1-\frac{3}{2}\frac{M_z}{\mu F_0 a}\right)^{\frac{1}{2}}\right]. \quad (6)$$

**Oscillating torsional moment**

The problem of elastic beads in Hertz contact subjected to oscillating torsional moment with fixed amplitudes $\pm M^*$ has been studied by Deresiewicz [3]. After the application of a moment $+M^*$, a decreasing moment leads to a reversal of slip at the edge of the contact circle with hysteresis in the angle of rotation. In a complete oscillation of the torsional moment a hysteresis loop is described, the area of which represents the energy dissipation per cycle [5].

The analytical developments of Deresiewicz [3] provide the relations for first increasing-moment, first decreasing-moment, and for the subsequent cycles. If the torsional moment oscillates between $\pm M^*$, the resultant angles of rotation are given by the following relations

$\mapsto$ decreasing torsional moment ($\frac{\partial M_z}{\partial t} < 0$) :

$$\overline{\beta}_d = \frac{Ga^2}{\mu F_0}\beta_d = \left[1-\frac{3}{4}\left(\overline{M}^*-\overline{M}\right)\right]^{\frac{1}{2}} - \frac{1}{2}\left[1+\left(1-\frac{3}{2}\overline{M}^*\right)^{\frac{1}{2}}\right] - \frac{3}{16}\overline{M}, \quad (7)$$

with $\overline{M} = \frac{M_0}{\mu F_0 a}$ and $\overline{M}^* = \frac{M^*}{\mu F_0 a}$;

$\mapsto$ increasing torsional moment ($\frac{\partial M_z}{\partial t} > 0$): $\beta_i = -\beta_d(-M_z)$

$$\overline{\beta}_i = \frac{Ga^2}{\mu F_0}\beta_i = -\left[1-\frac{3}{4}\left(\overline{M}^*+\overline{M}\right)\right]^{\frac{1}{2}} + \frac{1}{2}\left[1+\left(1-\frac{3}{2}\overline{M}^*\right)^{\frac{1}{2}}\right] - \frac{3}{16}\overline{M}. \quad (8)$$

Figure 3 shows the typical hysteresis loop associated to equations 7 and 8 when the torsional moment oscillates between $\pm M^*$.

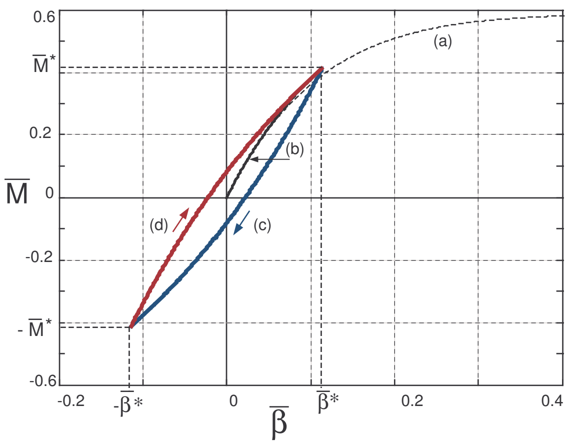


Figure 3. Curves illustrating torsional moment $\overline{M} = M_z/\mu F_0 a$ versus angle of rotation $\overline{\beta} = (Ga^2/\mu F_0)\beta$ during a complete cycle of applied moment. (a) : "exact" solution (Eq.5) and (b) : approximate solution Eq. (6). (c) and (d) : approximate relations Eq. (7) and Eq. (8) respectively.

### Nonlinear waves in a discrete chain of beads

It has shown above that, as the torsional moment oscillates, there is a region of slip occurring within the contact area, leading to nonlinear angle-torsional relations ($\beta = f(M_z)$) including the dependence on the history of the evolution (hysteretic behavior). For a rotational wave propagating in a discrete chain of elastic beads, the equation of motion of a bead $n$ can be written as

$$J\frac{\partial^2 \beta_n}{\partial t^2} = M_z(\beta_{n+1} - \beta_n) - M_z(\beta_n - \beta_{n-1}) \qquad (9)$$

where $J = \frac{2}{5}mR^2$ is the moment of inertia. $m$ and $R$ are, respectively, the mass and the radius of the beads. $\beta_n$ is the angle of rotation associated with the bead $n$.

We obtain a nonlinear torsional-angle relationship ($M_z = g(\beta)$) including hysteresis (characterized by the sign of $\partial\beta/\partial t$) by inverting the approximate relations of Deresiewicz, Eqs. (7-8). This relation is here expressed in a compact form :

$$\overline{M}sign(\dot{\beta}) = -\overline{M}^* - \frac{16}{3}\Big\{1 + B - \big(1 + 4B\big)^{\frac{1}{2}}\Big\}, \qquad (10)$$

with,

$$\overline{M}^* = -\frac{8}{3}\big[1 + 2\overline{\beta}^* - \big(1 + 8\overline{\beta}^*\big)^{\frac{1}{2}}\big], \qquad (11)$$

and $B = \overline{\beta}^* + \overline{\beta}.sign(\dot{\beta})$, where $\overline{M} = M_z/\mu F_0 a$, $\overline{\beta} = Ga^2/\mu N$, $\overline{\beta}^* = (Ga^2/\mu F_0)\beta^*$, and $\dot{\beta} = \partial\beta/\partial t$.

In this expression, the terms $(1 + X)^{\frac{1}{2}}$ are expanded in a power series of $X$ up to the quadratic term : $(1 + X)^{\frac{1}{2}} \simeq 1 + \frac{X}{2} - \frac{X^2}{8} + O(X^3)$. Finally, the torsional-angle relation, Eq. (10), reduces to the form,

$$\begin{aligned} M_z(\beta) &= M_z^{lin} + M_z^h \\ &\simeq K_t\Big\{\beta - h\big[\beta^*\beta + \frac{1}{2}(\beta^2 - \beta^{*2})sign\big(\dot{\beta}\big)\big]\Big\} \\ \text{with} \quad K_t &= \frac{dM_z}{d\beta} = \frac{16}{3}Ga^3 = (2R)(1-\nu).F_0, \\ \text{and} \quad h &= 4\frac{Ga^2}{\mu F_0} = \frac{2\,a^2 E}{\mu(1+\nu)F_0}, \end{aligned} \qquad (12)$$

where $K_t$ and $h$ are, respectively, the linear torsional rigidity and the parameter of quadratic hysteretic nonlinearity.

In contrast to the relations between stress and strain in a granular medium with Hertzian contact (under the action of normal and tangential forces), the Hertz nonlinearity (classical nonlinearity) is absent of this torsional-angle relation (obtained for small amplitudes of the applied moment). The only source of nonlinearities is hysteretic and it is due to the presence of circular slip at the contact surface.

### Wave equation with hysteretic nonlinearity

In this Section, we provide the calculation details for obtaining the evolution equation (3) of the article main text [7, 8]. To convert the discrete system (Eq. (9)) to a continuum approximation, it is assumed that the wavelength of the propagating waves is much larger than the distance between bead centers ($\lambda \gg 2R$). In this long wavelength regime, using a Taylor series expansion, the rotation angles $\beta_{n\pm1}$ can be expressed as

$$\beta_{n\pm1} = \beta_n \pm b\frac{\partial\beta_n}{\partial z} + \frac{b^2}{2!}\frac{\partial^2\beta_n}{\partial z^2} \pm \frac{b^3}{3!}\frac{\partial^3\beta_n}{\partial z^3} + \frac{b^4}{4!}\frac{\partial^4\beta_n}{\partial z^4} + O(b^5), \qquad (13)$$

where $b = 2R$ is the inter-bead spacing.

Neglecting terms of order higher than $O(b^4)$ and dispersive effects ($\partial^4\beta_n/\partial z^4$), the continuum form of the discrete equation (9) is reduced to the following wave equation (the index $n$ is deleted)

$$\frac{\partial^2\beta}{\partial t^2} - c^2\frac{\partial^2\beta}{\partial z^2} = -c^2\, h\,\frac{\partial T_h}{\partial\varphi}.\frac{\partial^2\beta}{\partial z^2} \qquad (14)$$

where $c = (2R)\sqrt{K_t/I}$ is the torsional wave velocity and $h$ the parameter of nonlinearity.

$$T_h = \varphi^*\varphi - \frac{1}{2}(\varphi^{*2} - \varphi^2).sign(\dot{\varphi}) \quad \text{with} \quad \varphi = (2R)\frac{\partial\beta}{\partial z} \tag{15}$$

is the term associated with the quadratic hysteretic nonlinearity.

The standard method of slowly varying wave profile (multiple scale technique) is now used to simplify Eq.(14) for progressive waves, assumed here to propagate in the $+z$ direction. The following coordinate transformation is introduced :

$$\beta = \epsilon\beta\big(\xi = \epsilon z\,; \tau = t - z/c\big),$$

where $\epsilon$ is a small parameter and $\tau$ a retarded time relative to a reference frame traveling at the wave velocity $c$.

With this coordinate change, we have,

$$\frac{\partial}{\partial\tau} \equiv \frac{\partial}{\partial t}, \quad \frac{\partial}{\partial z} \equiv \epsilon\frac{\partial}{\partial\xi} - \frac{1}{c}\frac{\partial}{\partial\tau}.$$

Using the above equalities in Eq. (14) and discarding terms of higher order than $\epsilon^2$ provides the first order equation with the variables $(z, \tau)$ :

$$\frac{\partial\varphi}{\partial z} + \frac{h}{2c}\frac{\partial T_h}{\partial\varphi}\frac{\partial\varphi}{\partial\tau} = 0. \tag{16}$$

### Angular particle velocity and normalization

With the relation,

$$\varphi = -\frac{2R}{c}\frac{\partial\beta}{\partial\tau},$$

the angular particle velocity

$$\theta_v = \frac{\partial\beta}{\partial\tau},$$

is introduced into Eq. (16), which gives,

$$\frac{\partial\theta_v}{\partial z} - \frac{h\,R}{c^2}\frac{\partial T'_h}{\partial\theta_v}\frac{\partial\theta_v}{\partial\tau} = 0 \tag{17}$$

with

$$T'_h = \theta_v^*\theta_v - \frac{1}{2}(\theta_v^{*2} - \theta_v^2)sign\big(\dot{\theta}_v\big).$$

The following dimensionless variables are introduced, $\overline{\theta}_v = \theta_v/\theta_0$ and $\tau' = \tau/\tau_0$ where $\theta_0$ is the amplitude and $\tau_0$ the characteristic duration of the first phase of the initial acoustic signal (in $z = 0$), and $\xi = z/z_{nl}$ with $z_{nl} = c^2\tau_0/2Rh\theta_0$ the characteristic nonlinear length. Then, the wave equation (17) can be rewritten in the form

$$\frac{\partial\overline{\theta}_v}{\partial\xi} - \frac{1}{2}\frac{\partial\overline{T}_h}{\partial\overline{\theta}_v}\frac{\partial\overline{\theta}_v}{\partial\tau'} = 0 \tag{18}$$

with

$$\overline{T}_h = \overline{\theta}_v^*\,\overline{\theta}_v - \frac{1}{2}(\overline{\theta}_v^{*2} - \overline{\theta}_v^2)sign\big(\dot{\overline{\theta}}_v\big).$$

### Step-wise linear approximation of wave profiles

This Section of Supplementary Materials is intended to provide more details on the derivation of the ordinary differential equations (4)-(6) from partial differential equation (3) of the article main text.

In normalized variables and functions, Eq. (3) takes the following form (identical to the one of Eq. (18) above),

$$\frac{\partial S}{\partial\xi} - \frac{1}{2}\frac{\partial M_h}{\partial S}\frac{\partial S}{\partial\tau} = 0, \tag{19}$$

where $M_h$ is the nonlinear part of the torsional moment, $S$ denotes the angular strain (or equivalently angular particle velocity for a different normalization), and $\partial M_h/\partial S$ corresponds to the normalized nonlinear torsional modulus. This equation is equivalent to the system of two ordinary differential equations

$$\frac{dS}{d\xi} = 0, \tag{20}$$

$$\frac{d\tau}{d\xi} = -\frac{1}{2}\frac{\partial M_h}{\partial S}, \tag{21}$$

which indicates that, when the wave propagation distance increases by $d\xi$, points of the wave profile $S = S(\tau, \xi)$ are displaced horizontally in the plane $(\tau, S)$ (see Fig. 4),

$$dS = 0\ , \quad d\tau = -\frac{1}{2}\frac{\partial M_h}{\partial S}d\xi. \tag{22}$$

Potentially, the rules in Eq. (22) provide a direct numerical routine to follow the evolution of an arbitrary wave profile for an arbitrary inhomogeneous distribution of the bi-stable hysteretic elements, hysterons, on the Preisach-Mayergoyz (PM) space [9–12]. The finger print of the hysteretic quadratic nonlinearity is known to be an homogeneous distribution of hysterons in the PM space [9].

This assumption is used here and is justified by the fact that we observed a quadratic hysteretic behavior of the contact in torsion (Fig. 2 of the main text). The symmetric preparation of the PM plane, i.e. a smoothed staircase separation along the diagonal of the PM plane in two regions with open and close hysteretic elements respectively is also assumed here. This situation is experimentally obtained by simply repeating the pulse generation several times before the signal recording. It is supposed to be produced by the previous pulse bouncing in the chain, interacting with the hysterons, and having a slowly decreasing amplitude until complete extinction.

In the particular case of interest here, the nonlinear hysteretic modulus is always negative and is equal to minus the length of the front closing (or opening) hysteretic elements on the PM plane (see illustration in Fig. A1). Thus in Eq. (22)), the condition $d\tau \geq 0$ is always fulfilled, corresponding to increasing time delay and stretching of the acoustic pulse with increasing propagation distance. Moreover for the homogeneous distribution of hysterons, $\partial M_h/\partial S$ is always a linear function of $S$. Because of this, if the boundary wave profile is approximated by a step-wise linear profile, then the profile after a propagation distance $d\xi$, obtained by the shifting rules (22), is again step-wise linear. To get an insight in the laws governing transformation of individual phases of a multi-phase acoustic pulse, it is sufficient to approximate the real profile by a step-wise linear profile, which is composed of straight segments connecting the extrema and the zero points $S = 0$ (Figs. 3 and 4 (a)). After the application of rules (22), a new single-valued profile [11, 13, 14] can be found at the distance $\xi + d\xi$ analytically and can be also approximated similarly. The shifts of individual phase extrema and the changes in the durations of the phases, caused by the propagation over distance $d\xi$, which are linear in small $d\xi$, are given in Eqs. (4)-(6).

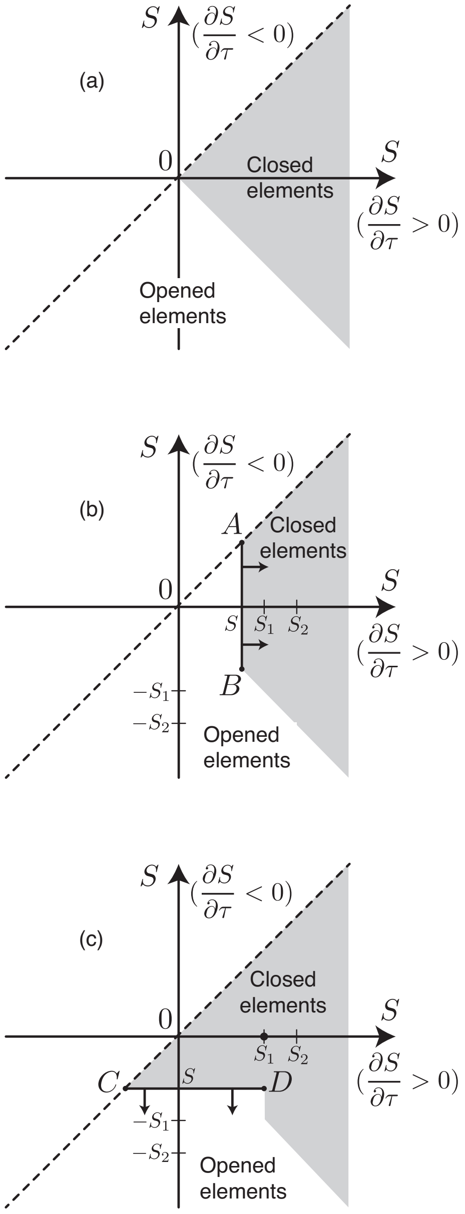


Figure 4. Evaluation of the nonlinear hysteretic modulus responsible for the transformation of the first leading phase of the acoustic pulse. (a) Initial distribution of opened and closed hysterons in the PM space. (b) The elastic modulus, corresponding to point $(\tau, S)$ of the leading front of the first phase is equal to minus the length of right-moving vertical segment AB, which opens the hysterons. (c) Elastic modulus, corresponding to point $(\tau, S)$ of the trailing front of the first phase is equal to minus the length of down-moving horizontal segment CD, which closes the hysterons.

---


[1] R. D. Mindlin. Compliance of elastic bodies in contact. *Trans. ASME, J. Appl. Mech.*, 71:259–268, 1949.

[2] J. L. Lubkin and P. H. McDonald. The torsion of elastic spheres in contact. *Trans. ASME, J. Appl. Mech.*, 18:183–187, 1951.

[3] H. Deresiewicz. Contact of elastic spheres under an oscillating torsional couple. *Trans. ASME, J. Appl. Mech.*, 21:52–56, 1954.

[4] M. Hetényi and P. H. McDonald. Contact stresses under combined pressure and twist. *Trans. ASME, J. Appl. Mech.*, 25:396–401, 1958.

[5] K.L. Johnson. *Contact mechanics*. Cambridge University

Press, Cambridge, 2nd edition, 1985.
[6] M. Abramowitz and I. A. Stegun. *Handbook of mathematical functions*. Dover publication, New York, 1972.
[7] V. Gusev, Wave Motion, 42, 97-108 (2005).
[8] V. Gusev, Wave Motion 33, 145-153 (2001).
[9] R.A. Guyer and P.A. Johnson, *Nonlinear Mesoscopic Elasticity*, (WILEY-VCH, 2009).
[10] V. Gusev and V. Aleshin, J. Acoust. Soc. Am. 112, 2666 (2002).
[11] V. Aleshin, V. Gusev, V. Zaitsev, Ultrasonics 42, 1053-1059 (2004).
[12] V. Aleshin, V. Gusev, V. Zaitsev, J. Computational Acoustics 12, 319-354 (2004).
[13] V. Gusev, Acta Acustica United with Acustica 89, 445-450 (2003).
[14] V. Gusev, W. Lauriks, C. Glorieux and J. Thoen, Phys. Lett. A 232, 77-86 (1997).
[15] V. Gusev and V. Zaitsev, Phys. Lett. A 314, 117-125 (2003).
[16] V.Yu. Zaitsev, V. Gusev, Yu.V. Zaytsev, Ultrasonics 43, 699-709 (2005).
